# Supplementary material for: Forensic Self-Descriptions Are All You Need for Zero-Shot Detection, Open-Set Source Attribution, and Clustering of AI-generated Images
Source: arXiv:2503.21003 source file (2025-03-26)
Supplement: Supplementary file 1 [file ClusteringByArchFamily_v0.tex]

\section{Clustering by Generative Model Family}
\label{supp:clustering_by_arch_fam}
