# Supplementary material for: Forensic Self-Descriptions Are All You Need for Zero-Shot Detection, Open-Set Source Attribution, and Clustering of AI-generated Images
Source: arXiv:2503.21003 source file (2025-03-26)
Supplement: Supplementary file 2 [file RobustnessResults_v0.tex]

\section{Robustness to Post Processing and Social Media Compression}
\label{supp:robustness}
